# Supplementary material for: Rotation Invariant Convolutions for 3D Point Clouds Deep Learning
Source: arXiv:1908.06297 source file (2019-08-17)
Supplement: Supplementary file 1 [file supp.pdf]

# Rotation Invariant Convolutions for 3D Point Clouds Deep Learning
# Supplementary Material

Zhiyuan Zhang[1] Binh-Son Hua[2] David W. Rosen[1] Sai-Kit Yeung[3]

[1]Singapore University of Technology and Design [2]The University of Tokyo
[3]Hong Kong University of Science and Technology

## Abstract

*In this supplementary document, we provide more details about the quantitative and qualitative evaluations presented in the main paper [6]. Particular, we detail convergence plot of testing accuracy/mIoU score over training epochs in the classification and part segmentation task, respectively, to demonstrate the efficiency of our rotation invariance convolution. We report both results in the z/SO3 scenario which is the most challenging case in evaluating rotation invariance convolution. In addition, we also report per-class accuracy in the classification task, and add more visualization results in the object part segmentation task.*

## 1. Object Classification

To further demonstrate the benefit of our proposed convolution, we plot the evaluation accuracy against training epochs. The results are shown in Figure 1. In addition, we report per-class accuracy of the classification task in Table 1. As can be seen, we outperforms previous methods significantly. The results of PointCNN [1] is the closest to ours, but in some categories, e.g., desk, laptop, mantel, etc., the results are still less than 50% despite that their convolution also learns a latent transformation. PointNet-based techniques [2, 3] also perform poorly even there are a transformation network learned to rotate the input points into a standard pose. This z/SO3 scenario shows that such transformation networks do not generally adapt well to unseen rotated data.

## 2. Object Part Segmentation

For object part segmentation task, we also detail the capability of generalizing to unseen rotations in our method by plotting the testing mIoU score at different training epochs. The results are in Figure 2. Similar to the observation in the object classification task, it can be seen that our method outperforms previous methods significantly even at early

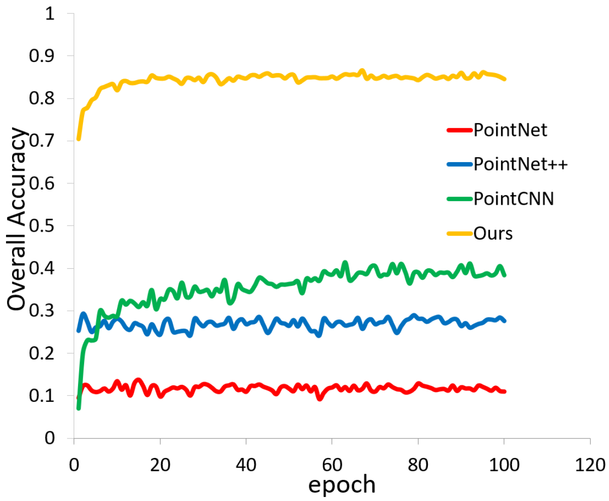


Figure 1. Overall accuracy vs. epochs plot of object classification with z/SO3 scenario. Our method (yellow) is better than PointCNN [1] (green) $\approx$ 10% of accuracy even with early epochs.

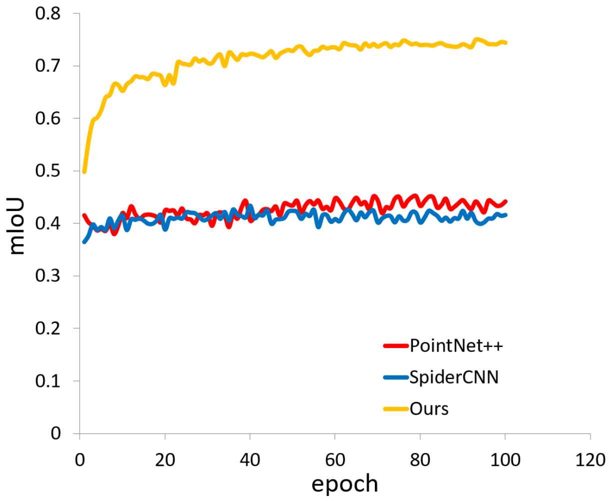


Figure 2. mIoU vs. epochs plot of object part segmentation with z/SO3 scenario. Our rotation invariance convolution outperforms state-of-the-art point cloud learning [3, 5] significantly.

| Network | airplane | bathtub | bed | bench | bookshelf | bottle | bowl | car | chair | cone |
|---|---|---|---|---|---|---|---|---|---|---|
| PointNet [2] | 12.0 | 2.0 | 8.0 | 10.0 | 15.0 | 14.0 | 5.0 | 12.0 | 9.0 | 15.0 |
| PointNet++ [3] | 53.0 | 2.0 | 18.0 | 10.0 | 29.0 | 22.0 | 20.0 | 13.0 | 32.0 | 20.0 |
| PointCNN [1] | 60.0 | 10.0 | 20.0 | 10.0 | 20.0 | 37.0 | 25.0 | 34.0 | 46.0 | 25.0 |
| Ours | **100.0** | **82.0** | **94.0** | **80.0** | **93.0** | **94.0** | **100.0** | **98.0** | **96.0** | **90.0** |
| | cup | curtain | desk | door | dresser | flower pot | glass box | guitar | keyboard | lamp |
| PointNet[2] | 0.0 | 0.0 | 16.3 | 5.0 | 8.1 | 0.0 | 4.0 | 36.0 | 5.0 | 15.0 |
| PointNet++ [3] | 15.0 | 45.0 | 2.3 | 30.0 | 9.3 | 15.0 | 11.0 | 47.0 | 50.0 | 10.0 |
| PointCNN [1] | 15.0 | 40.0 | 34.9 | 30.0 | 32.6 | 25.0 | 35.0 | 46.0 | 50.0 | 20.0 |
| Ours | **60.0** | **95.0** | **79.1** | **85.0** | **73.3** | **30.0** | **96.0** | **99.0** | **95.0** | **80.0** |
| | laptop | mantel | monitor | night stand | person | piano | plant | radio | range hood | sink |
| PointNet [2] | 15.0 | 4.0 | 11.0 | 3.5 | 5.0 | 36.7 | 55.0 | 5.0 | 4.0 | 20.0 |
| PointNet++ [3] | 15.0 | 10.0 | 36.0 | 1.2 | 20.0 | 5.0 | 71.0 | 20.0 | 9.0 | 5.0 |
| PointCNN [1] | 20.0 | 38.0 | 35.0 | 40.7 | 15.0 | 34.0 | 26.0 | 10.0 | 28.0 | 20.0 |
| Ours | **95.0** | **91.9** | **97.0** | **77.9** | **85.0** | **90.8** | **83.0** | **55.0** | **87.0** | **75.0** |
| | sofa | stairs | stool | table | tent | toilet | tv stand | vase | wardrobe | xbox |
| PointNet [2] | 11.0 | 25.0 | 5.0 | 3.0 | 5.0 | 20.0 | 4.0 | 26.3 | 0.0 | 10.0 |
| PointNet++ [3] | 21.0 | 10.0 | 10.0 | 9.0 | 15.0 | 13.0 | 2.0 | **85.0** | 15.0 | 20.0 |
| PointCNN [1] | 32.0 | 30.0 | 20.0 | 36.0 | 15.0 | 33.0 | 29.0 | 70.0 | 40.0 | 15.0 |
| Ours | **92.0** | **85.0** | **60.0** | **80.0** | **70.0** | **95.0** | **78.0** | 76.8 | **70.0** | **65.0** |

Table 1. Per-class accuracy of object classification in z/SO3 scenario with the ModelNet40 dataset [4].

epochs.

Additional visualizations of object part segmentation in shown in Figure 3.

## References


[1] Y. Li, R. Bu, M. Sun, and B. Chen. Pointcnn: Convolution on x-transformed points. *Advances in Neural Information Processing Systems*, 2018. 1, 2

[2] C. R. Qi, H. Su, K. Mo, and L. J. Guibas. Pointnet: Deep learning on point sets for 3d classification and segmentation. In *CVPR*, 2017. 1, 2

[3] C. R. Qi, L. Yi, H. Su, and L. J. Guibas. Pointnet++: Deep hierarchical feature learning on point sets in a metric space. In *Advances in Neural Information Processing Systems*, pages 5105–5114, 2017. 1, 2

[4] Z. Wu, S. Song, A. Khosla, F. Yu, L. Zhang, X. Tang, and J. Xiao. 3d shapenets: A deep representation for volumetric shapes. In *CVPR*, pages 1912–1920, 2015. 2

[5] Y. Xu, T. Fan, M. Xu, L. Zeng, and Y. Qiao. Spidercnn: Deep learning on point sets with parameterized convolutional filters. In *ECCV*, 2018. 1

[6] Z. Zhang, B.-S. Hua, D. W. Rosen, and S.-K. Yeung. Rotation invariant convolutions for 3d point clouds deep learning. In *International Conference on 3D Vision (3DV)*, 2019. 1

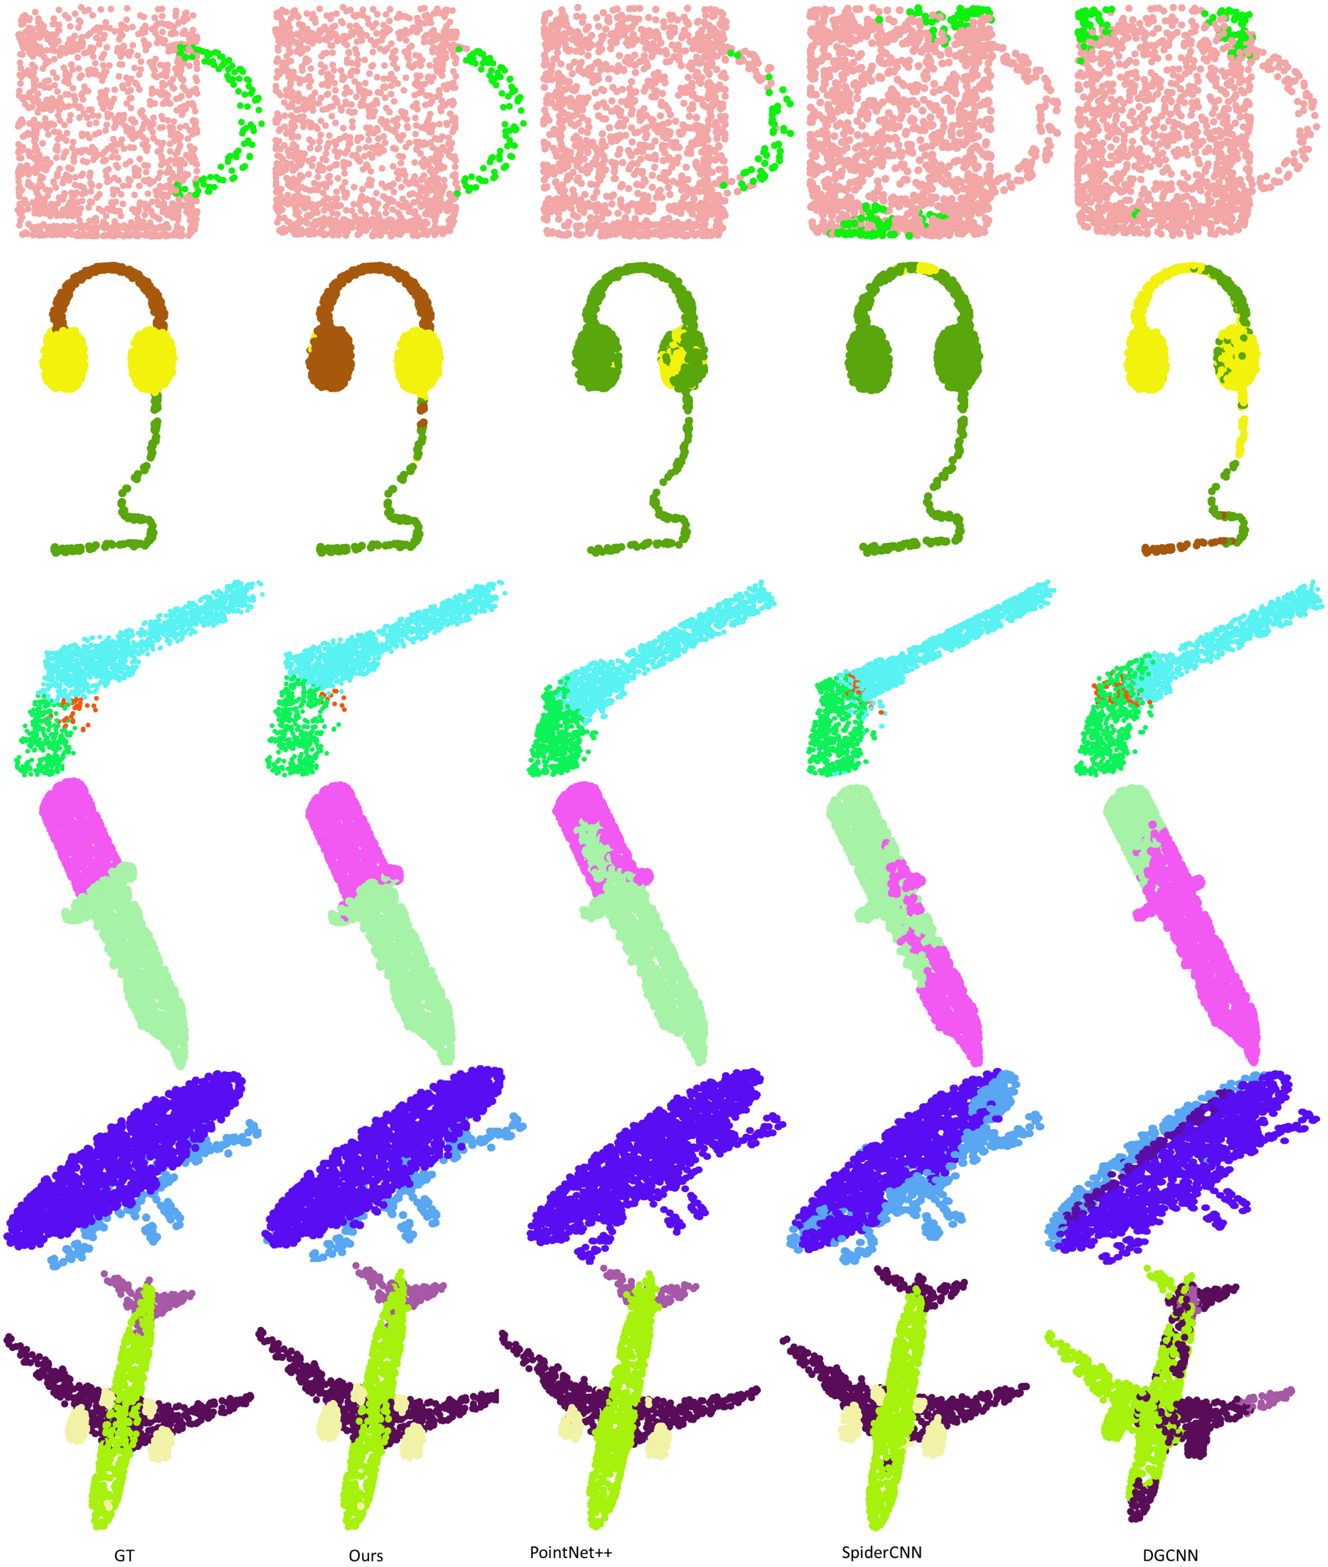


Figure 3. Additional qualitative results of object part segmentation task with z/SO3 scenario. Our method has the state-of-the-art performance while previous methods fail to generalize to SO3 rotations.
